# Supplementary material for: Assessing and Verifying Task Utility in LLM-Powered Applications
Source: arXiv:2405.02178 source file (2024-05-12)
Supplement: Supplementary file 1 [file appendix_related_work.tex]

\subsection{LLMs as Evaluators}
Recent work has began looking at the potential of LLMs as evaluators. \citeauthor{chan2023chateval} propose ChatEval, a multi-agent referee team that discusses and evaluates responses from agents on open-ended generation tasks (debate-style), leading to text that aligns with better human preferences. \citeauthor{chern2024can} also propose a multiple agent-debate-assisted meta-evaluation framework, which can make human annotation easier.  \citeauthor{wang2023chatgpt} explore if ChatGPT itself can be used as an evaluator, by prompting it to score texts. \citeauthor{chiang2023can} propose that LLMs can be used to assess the quality of texts, by comparing to human rated texts. Other works identify weaknesses in LLMs as evaluators, and propose to improve them, such as the multi-step calibration framework proposed by \citeauthor{wang2023large}. In contrast, we propose to use multiple LLMs, where each has a defined task, leading to better task evaluation.
